# Supplementary material for: Fast training of accurate physics-informed neural networks without gradient descent
Source: arXiv:2405.20836 source file (2026-04-15)
Supplement: Supplementary file 1 [file fenics.tex]

%%%%%%%%%
% Fenics details go ahere! 
%%%%%%%%%%
